# Supplementary material for: Misspecification of Multiple Scattering in Scalar Wave Fields and its Impact in Ultrasound Tomography
Source: arXiv:2405.01220 source file (2024-10-01)
Supplement: Supplementary file 1 [file appendix_a.tex]

\subsection{Proof of \Cref{th_slepian}} \label{appendix_a}
Recall that the MLL of the considered complex Gaussian model with misspecified mean is given by
\begin{align*}
	v = - \ln(\pi^N \text{det}\{ \bm{\Sigma} \}) - (\bm{y} - \bm{\mu})\herm \bm{\Sigma}^{-1} (\bm{y} - \bm{\mu}),
\end{align*}
where the true model $p_Y(\bm{y})$ for $\bm{y} \in \compl^N$ is given by $\mathcal{CN}(\bm{s}, \bm{\Sigma})$ and the misspecified model $f_Y(\bm{y} \vert \bm{\theta})$ is given by $\mathcal{CN}(\bm{\mu}, \bm{\Sigma})$. The misspecified mean $\bm{\mu} = \bm{\mu}(\bm{\theta})$ is a function $\bm{\mu} : \real^d \to \compl^N$. Furthermore, the noise covariance $\bm{\Sigma}$ is taken to be real-valued. Based on \cref{def_MLL,def_MCRB}, the gradient and Hessian of the MLL are required to compute the matrices $\bm{A}_{\bm{\theta}_0}$ and $\bm{B}_{\bm{\theta}_0}$ from which the MCRB is defined. 

Noting that the noise covariance matrix $\bm{\Sigma}$ is independent from the parameters $\theta_i$, $\bm{\theta} = [\theta_i]_{i=1}^d$, an element of the gradient of the MLL is given by
\begin{align}
\begin{gathered}
	\frac{\partial v}{\partial \theta_i} = -\frac{\partial (\bm{y} - \bm{\mu})\herm}{\partial \theta_i} \bm{\Sigma}^{-1} (\bm{y} - \bm{\mu}) + \\ 
	(\bm{y} - \bm{\mu})\herm \bm{\Sigma}^{-1} \left( \frac{\partial \bm{\mu}}{\partial \theta_i} \right).
\end{gathered}
\end{align}
The derivatives are considered only in the real sense. Under these conditions, one obtains
\begin{align}
\begin{gathered}
	\frac{\partial v}{\partial \theta_i} = \left( \frac{\partial\bm{\mu}}{\partial \theta_i} \right)\herm \bm{\Sigma}^{-1} (\bm{y} - \bm{\mu}) +  
	(\bm{y} - \bm{\mu})\herm \bm{\Sigma}^{-1} \left( \frac{\partial \bm{\mu}}{\partial \theta_i} \right) = \\
	2 \text{Re} \left\{ \left( \frac{\partial\bm{\mu}}{\partial \theta_i} \right)\herm \bm{\Sigma}^{-1} (\bm{y} - \bm{\mu}) \right\}.
\end{gathered}
\label{eq_grad}
\end{align}
Following a similar procedure, \eqref{eq_hess} is obtained.

From equation \eqref{eq_A}, evaluating at the PTS $\bm{\theta}_0$ and taking the expectation of \eqref{eq_hess} with respect to the true PDF yields $\bm{A}_{\bm{\theta}_0}$. All quantities in \eqref{eq_hess} are deterministic save for $\bm{y}$, which obeys $\bm{y} = \bm{s} + \bm{n}$ and $\bm{n} \sim \mathcal{CN}(\bm{0}, \bm{\Sigma})$ according to the true model. Furthermore, for a complex random variable $z$, note that {$\mathbb{E} \{ \text{Re} \{ z \} \} = \text{Re} \{ \mathbb{E} \{ z \} \}$} due to linearity of the expectation and its commutativity with complex conjugation. Exploiting these properties, the first of the Slepian formulae is found to be
\begin{align*}
\begin{gathered}
	[\bm{A}_{\bm{\theta}_0}]_{ij} = 2 \text{Re} \Bigg\{ \mathbb{E}_p \Bigg\{  - \left( \frac{\partial\bm{\mu}}{\partial \theta_j} \right)\herm \bm{\Sigma}^{-1} \left( \frac{\partial\bm{\mu}}{\partial \theta_i} \right) + \\
	\left( \frac{\partial^2 \bm{\mu}}{\partial \theta_i \theta_j} \right)\herm \bm{\Sigma}^{-1} (\bm{y} - \bm{\mu}) \Bigg\vert_{\bm{\theta} = \bm{\theta}_0} \Bigg\} \Bigg\} \\
\end{gathered}
\end{align*}
which yields
\begin{align}
\begin{gathered}
	[\bm{A}_{\bm{\theta}_0}]_{ij} =  2 \text{Re} \Bigg\{ - \left( \frac{\partial\bm{\mu}}{\partial \theta_j} \right)\herm \bm{\Sigma}^{-1} \left( \frac{\partial\bm{\mu}}{\partial \theta_i} \right) + \\
	\left( \frac{\partial^2 \bm{\mu}}{\partial \theta_i \theta_j} \right)\herm \bm{\Sigma}^{-1} (\bm{s} - \bm{\mu}) \Bigg\vert_{\bm{\theta} = \bm{\theta}_0} \Bigg\}. \\
	\hfill \blacksquare
\end{gathered}
\end{align}

Regarding the $\bm{B}_{\bm{\theta}_0}$ matrix, the expectation of the product of two terms of the form \eqref{eq_grad} is required. With appropriate substitutions, the partial derivative in \eqref{eq_grad} evaluated at $\bm{\theta}_0$ can be rewritten as
\begin{align}
\begin{gathered}
	\left( \frac{\partial v}{\partial \theta_i} \right) \Bigg\vert_{\bm{\theta} = \bm{\theta}_0} = a + a^*
\end{gathered}
\end{align}
for a complex number $a$. Applying this notation to \eqref{eq_B}, the expression
\begin{align}
\begin{gathered}
	[\bm{B}_{\bm{\theta}_0} ]_{ij} = \mathbb{E}_p \left\{ \left( \frac{\partial v}{\partial \theta_i} \right) \left( \frac{\partial v}{\partial \theta_j} \right)\Bigg\vert _{\bm{\theta}=\bm{\theta}_0} \right\} = \\
	\mathbb{E}_p \left\{ (a + a^*)(b + b^*) \right\} = 2 \text{Re} \{ \mathbb{E}_p \left\{ ab + a^*b \right\} \}
\end{gathered}
\end{align}
is obtained, where, after conjugating and transposing as needed,
\begin{align}
	a = (\bm{y} - \bm{\mu}) \herm \bm{\Sigma}^{-1} \left( \frac{\partial\bm{\mu}}{\partial \theta_i} \right) \Bigg\vert_{\bm{\theta} = \bm{\theta}_0}
\end{align}
and
\begin{align}
	b = (\bm{y} - \bm{\mu}) \herm \bm{\Sigma}^{-1} \left( \frac{\partial\bm{\mu}}{\partial \theta_j} \right) \Bigg\vert_{\bm{\theta} = \bm{\theta}_0}.
\end{align}

{After rearranging}, only the product $(\bm{y} - \bm{\mu})^*(\bm{y} - \bm{\mu})\herm$ is found to be stochastic. Expanding $\bm{y} = \bm{s} + \bm{n}$ and substituting $\bm{w} = \bm{s} - \bm{\mu}$, the difference $\bm{y} - \bm{\mu}$ is rewritten as $\bm{w} + \bm{n}$, where $\bm{w}$ is deterministic. Additionally, due to the circular symmetry of $\bm{n}$, $\mathbb{E}_p \{ \bm{n} \bm{n}\trans \} = \bm{0}_N$, where $\bm{0}_N$ is a zero matrix of size $N \times N$. It follows that
\begin{align}
\begin{gathered}
	\mathbb{E}_p \{ (\bm{y} - \bm{\mu})^*(\bm{y} - \bm{\mu})\herm \} = \\
	\bm{w}^*\bm{w}\herm = (\bm{s} - \bm{\mu})^* (\bm{s} - \bm{\mu})\herm,
\end{gathered}
\end{align}
and thus
\begin{align}
\begin{gathered}
	\mathbb{E}_p \left\{ ab \right\} = \mathbb{E}_p \left\{ a\trans b \right\} = \\ 
	\left( \frac{\partial \bm{\mu}}{\partial \theta_i} \right)\trans \bm{\Sigma}^{-1} (\bm{s} - \bm{\mu})^* (\bm{s} - \bm{\mu})\herm \bm{\Sigma}^{-1} \left( \frac{\partial \bm{\mu}}{\partial \theta_j} \right) \Bigg\vert _{\bm{\theta}=\bm{\theta}_0}.
\end{gathered}
\end{align}
{This procedure is repeated for $a^*b = a\herm b$, yielding}
\begin{align}
\begin{gathered}
	\mathbb{E}_p \{ (\bm{y} - \bm{\mu})(\bm{y} - \bm{\mu})\herm \} = \\
	\bm{w}\bm{w}\herm + \mathbb{E}_p \{ \bm{n}\bm{n}\herm \} = (\bm{s} - \bm{\mu}) (\bm{s} - \bm{\mu})\herm + \bm{\Sigma},
\end{gathered}
\end{align}
so that
\begin{align}
\begin{gathered}
	\mathbb{E}_p \left\{ a^* b \right\} = \mathbb{E}_p \left\{ a\herm b \right\} = \\
	\left( \frac{\partial \bm{\mu}}{\partial \theta_i} \right)\trans \bm{\Sigma}^{-1} (\bm{s} - \bm{\mu}) (\bm{s} - \bm{\mu})\herm \bm{\Sigma}^{-1} \left( \frac{\partial \bm{\mu}}{\partial \theta_j} \right) + \\
	\left( \frac{\partial \bm{\mu}}{\partial \theta_i} \right)\trans \bm{\Sigma}^{-1} \bm{\Sigma} \bm{\Sigma}^{-1} \left( \frac{\partial \bm{\mu}}{\partial \theta_j} \right) \Bigg\vert _{\bm{\theta}=\bm{\theta}_0}.
\end{gathered}
\end{align}
Based on these results, the second of the Slepian formulae takes the form
\begin{align}
\begin{gathered}
	[\bm{B}_{\bm{\theta}_0} ]_{ij} = 2 \text{Re} \{ \mathbb{E}_p \left\{ ab + a^*b \right\} \} = 2\text{Re} \Bigg\{ \\
	\left( \frac{\partial \bm{\mu}}{\partial \theta_i} \right)\trans \bm{\Sigma}^{-1} (\bm{s}-\bm{\mu})^* (\bm{s}-\bm{\mu})\herm \bm{\Sigma}^{-1} \left( \frac{\partial \bm{\mu}}{\partial \theta_j} \right) + \\
	\left( \frac{\partial \bm{\mu}}{\partial \theta_i} \right)\herm \bm{\Sigma}^{-1} (\bm{s}-\bm{\mu}) (\bm{s}-\bm{\mu})\herm \bm{\Sigma}^{-1} \left( \frac{\partial \bm{\mu}}{\partial \theta_j} \right) + \\
	\left( \frac{\partial \bm{\mu}}{\partial \theta_i} \right)\herm \bm{\Sigma}^{-1} \left( \frac{\partial \bm{\mu}}{\partial \theta_j} \right) \Bigg\vert _{\bm{\theta}=\bm{\theta}_0}	\Bigg\}. \\
	\hfill \blacksquare
\end{gathered}
\end{align}
